# Supplementary material for: QUART-Online: Latency-Free Large Multimodal Language Model for Quadruped Robot Learning
Source: arXiv:2412.15576 source file (2025-05-27)
Supplement: Supplementary file 1 [file exps_additional_capabilities.tex]

\subsection{Additional LLM Capabilities} \label{app:additional_capabilities}

Using a large pretrained LLM also means we can leverage its capabilities beyond code-writing.
For example, Code as Policies can parse commands from non-English languages as well as emojis.
See Figure~\ref{fig:additional_capabilities}.

% \begin{figure}[t]
%     \centering
%     \includegraphics[width=\linewidth]{ims/additional_capabilities.png}
%     \caption{
%     \footnotesize
%     LMPs inherit benefits of LLMs, such as parsing commands from non-English languages and emojis.
%     }
%     \label{fig:additional_capabilities}
% \end{figure}
